# Supplementary material for: Learning Geometry-Guided Depth via Projective Modeling for Monocular 3D Object Detection
Source: arXiv:2107.13931 source file (2024-04-24)
Supplement: Supplementary file 1 [file Appendix.tex]

%%%%%%%%% BODY TEXT - ENTER YOUR RESPONSE BELOW
\newpage
\setcounter{section}{0}

%-------------------------------------------------------------------------

\section{Additional results on the test set for the car category with the metric of $AP_{11}$}
As mentioned in the main paper, we report the performance of existing works on the KITTI 3D \emph{test} and \emph{validation} sets for the car category with the evaluation metric of $AP_{40}$, following MonoDIS~\cite{monodis}. 
To better compare our approach with other methods, we further report results on on the KITTI 3D 
% \emph{test} and 
\emph{validation} sets for the car category with the evaluation metric of $AP_{11}$. 
As represented in Table~\ref{tb: val 11}, the KITTI validation results in terms of the metric of $AP_{11}$ are quoted from the MonoPair~\cite{monopair}. Our approach achieves a notable improvement over the state-of-the-art monocular image-based detectors on 
\emph{validation} set with the evaluation metric of $AP_{11}$. 
Our approach achieves 23.21\% ($0.95\%$ improvement) on the easy, 19.67\% ($ 1.25\%$ improvement) on the moderate, and 17.21\% ($ 0.72\%$ improvement) on the hard compared with the previous state-of-the-art image-only method for 3D object detection.
For the Bird’s Eye View (BEV) on the car class, our method also achieves the best performance, increasing the $AP_{40}$ over the second best method by $1.7\%$, $1.10\%$, $1.36\%$ on the easy moderate, and hard level, respectively.

%-------------------------------------------------------------------------

\section{Further Analysis on Depth Estimation from Geometry}
We also show Depth statistics on the training set. Table~\ref{tb: analysis_loc_error} shows that for two cars with the same height in both the 2D bounding box and the 3D bounding box, the depth values of their centers differ by more than $5$ meters because of their distinct \emph{poses} and \emph{locations}.
This shows the necessity of considering 3D pose and position for geometric formula, which is not considered by previous works.

\begin{table}[!thb]
\begin{center}
\resizebox{1\linewidth}{!}
{
\begin{tabular}{c|c |c cccc}
\toprule
\multicolumn{1}{l|}{\multirow{2}{*}{$h$}} &\multirow{2}{*}{dep.}
	&\multicolumn{5}{c}{The Height of 3D bounding boxes}\\
\cline{3-7}
    &   & avg.  & $1.49m$  &$1.50m$  & $1.51m$  & $1.52m$  \\
% 	& 	&avg.  & 1.39m  & 1.45m  & 1.51m  & 1.57m  & 1.63m  \\
\hline
\multirow{3}{*}{30}               
                    & $\max$                    & 39.51 & 40.23 & 40.39 & 42.23 & 39.47 \\
% \cline{3-7}
                    & $\min$                    & 37.69 & 36.53 & 36.53 & 37.21 & 37.25 \\
% \cline{3-7}
                    & diff.                     & 1.82  & 3.70  & 3.86  & 5.02  & 2.22  \\
\hline
\multirow{3}{*}{35}              
                    & $\max$                    & 34.04 & 34.68 & 35.69 & 34.12 & 36.40 \\
% \cline{3-7}
                    & $\min$                    & 32.99 & 31.72 & 31.77 & 32.05 & 31.75 \\
% \cline{3-7}
                    & diff.                     & 1.05  & 2.96  & 3.92  & 2.07  & 4.65  \\
\bottomrule
\end{tabular}
}
\end{center}
\caption{ \textbf{Depth values on training set (in meter).} We show the maximum (max) and minimum (min) depth values of the cars with the same height of 2D bounding box $h$ and the same height of 3D bounding box (in different columns). The difference (diff.) between the maximum and minimum depth values are also shown.
}
\label{tb: analysis_loc_error}
\end{table}

%-------------------------------------------------------------------------

\section{Additional Qualitative Results and Depth Visualization}

We also present additional visualization of the prediction results on KITTI 3D raw data in both Image plane and LiDAR coordinate system. We provide further visualization of the 
% geometry features
depth estimation, including depth from geometry formula and final depth output. A video with those results is available in the supplementary directory. 
The predictions in image plane and in LiDAR coordinate and the visualization of depth estimation are shown in each figure from top to down. And in the visualization of depth estimation, we show the depth from the geometry formula in the left and the final depth output in the right.
The red solid lines in LiDAR coordinate system represent the visible range  on the image. And the orange boxes mean predictions from cars. In the visualization of depth estimation, we use JET Color map Type in openCV, where scene depth values from small to large corresponds to the color from blue to red.
More results are also available in the video.

Depth estimation is a critical performance bottleneck in the monocular 3D object detection as mentioned in the main paper.  The depth from the geometry formula shows a great ability to estimate stably and accurately. Compared with the final depth output, the depth estimation from the our proposed geometry formula will not change drastically when new vehicles appears or vehicles move. The proposed geometry module from the 2D/3D information provides more reliable depth estimation for more accurate predictions.

%-------------------------------------------------------------------------

\begin{table*}[!htp]
\begin{center}
\resizebox{1.\linewidth}{!}
{
%\begin{tabular}{l | c |ccc |ccc |ccc|ccc}
\begin{tabular}{l |ccc |ccc |ccc|ccc}
\toprule
\multirow{2}{*}{Method}	
%&\multirow{2}{*}{Modality}	
&\multicolumn{3}{c|}{3D Detection IoU$\geq$0.7}		&\multicolumn{3}{c|}{BEV IoU$\geq$0.7} &\multicolumn{3}{c|}{3D Detection IoU$\geq$0.5}		&\multicolumn{3}{c}{BEV IoU$\geq$0.5}\\
\cline{2-13}
						&Easy &Mod. &Hard 			&Easy &Mod. &Hard
						&Easy &Mod. &Hard 			&Easy &Mod. &Hard\\
\hline\hline 
Mono3D~\cite{chen20153d}      
            & 2.53  & 2.31  & 2.31  
            & 5.22  & 5.19  & 4.13  
            & 25.19 & 18.20 & 15.52 
            & 30.50 & 22.34 & 19.16 \\
OFTNet~\cite{oftnet}      
            & 4.07  & 3.27  & 3.29  
            & 11.06 & 8.79  & 8.91  
            & -     & -     & -     
            & -     & -     & -     \\
MF3D~\cite{mf3d}      
            & 10.53 & 5.69  & 5.39  & 22.03 & 13.63 & 11.60 & 47.88 & 29.48 & 26.44 & 55.02 & 36.73 & 31.27 \\
MonoPSR~\cite{monopsr}   
            & 12.75 & 11.48 & 8.59  & 20.63 & 18.67 & 14.45 & 47.88 & 29.48 & 26.44 & 56.97 & 43.39 & 36.00 \\
TLNet (mono)~\cite{tlnet}
            & 13.77 & 9.72  & 9.29  & 21.91 & 15.72 & 14.32 & 49.65 & 41.71 & 29.95 & 52.72 & 37.22 & 32.16 \\
MonoGRNet~\cite{monogrnet}   
            & 13.88 & 10.19 & 7.62  & 24.97 & 19.44 & 16.30 & 48.34 & 33.98 & 28.67 & 54.21 & 39.69 & 33.06 \\
MonoDIS~\cite{monodis}     
            & 18.05 & 14.98 & 13.42 & 24.26 & 18.43 & 16.95 & /     & /     & /     & /     & /     & /     \\
M3D-RPN~\cite{m3drpn}     
            & 20.27 & 17.06 & 15.21 & 25.94 & 21.18 & 17.90 & 50.51 & 36.97 & 30.82 & 55.37 & 42.49 & 35.29 \\
MonoPair~\cite{monopair}				
						&\boldblue{22.26}
						&\boldblue{18.42}
						&\boldblue{16.49}
						&\boldblue{28.97}
						&\boldblue{22.65}
						&\boldblue{21.10}
						&\boldblue{55.88}
						&\boldblue{43.32}
						&\boldblack{40.94}
						&\boldblue{59.66}
						&\boldblack{49.52}
						&\boldblack{43.76} \\
\hline\hline
Baseline    & 19.90 & 16.23 & 14.02 & 27.08 & 19.86 & 18.83 
            & 54.57 & 40.85 & 39.08 & 58.44 & 46.95 & 41.37 \\
Our method				&\textbf{23.21}	&\textbf{19.67}	&\textbf{17.21}	
						&\textbf{30.67}	&\textbf{23.75}	&\textbf{22.46}	
						&\textbf{57.00}	&\textbf{43.41}	&\boldblue{40.89}	
						&\textbf{60.04}	&\boldblue{49.40}	&\boldblue{43.58}\\
\bottomrule
\end{tabular}
}
\end{center}
\caption{
\textbf{Monocular 3D object detection results on the KITTI {\textit{validation}} set} for the car category with the evaluation metric of $AP_{11}$. The results of the previous works are from~\cite{monopair}. Our approach significantly outperforms the previous state-of-the-arts on almost all the different evaluation protocols and settings. The bold \textbf{black}/\boldblue{blue} color indicates the best/the second best performing method.}
\label{tb: val 11}
\end{table*}

%-------------------------------------------------------------------------

\begin{figure*}[!t]
\begin{center}
\includegraphics[width=0.95\linewidth]{figure/d6-0000000270.png}
\end{center}
   \caption{
   \textbf{Qualitative Results and Depth Visualization}
The predictions in image plane and in LiDAR coordinate and the visualization of depth estimation are shown in from top to down. 
And in the visualization of depth estimation, we show the depth from the geometry formula in the left and the final depth output in the right.
The red solid lines in LiDAR coordinate system represent the visible range  on the image. And the orange boxes mean predictions for the car category.}
\label{fig: framework}
\end{figure*}
